# Supplementary material for: Introduction and Exemplars of Uncertainty Decomposition
Source: arXiv:2211.15475 source file (2022-11-17)
Supplement: Supplementary file 1 [file appendix.tex]

Additional material goes here
